# Supplementary material for: TensorCodec: Compact Lossy Compression of Tensors without Strong Data Assumptions
Source: arXiv:2309.10310 source file (2023-09-20)
Supplement: Supplementary file 1 [file 7appendix.tex]

\begin{comment}
\begin{table}[t]
    \centering
    \caption{Sizes of tensors used in Figure~\ref{fig:scalable:train}} \label{tab:syntensor} 
    \scalebox{0.8}
    {
        \begin{tabular}{c|l}
        \toprule
        Order & Size of Tensor \\
        \midrule
         \multirow{5}{*}{3} & $256 \times 256 \times 128$  \\
         & $256 \times 256 \times 256$ \\
         & $512 \times 256 \times 256$ \\
         & $512 \times 512 \times 256$ \\
         & $512 \times 512 \times 512$ \\
         \bottomrule         
        \end{tabular}
        
        \begin{tabular}{c|l}
        \toprule
        Order & Size of Tensor \\
        \midrule
        \multirow{5}{*}{4} & $64 \times 64 \times 64 \times 64$ \\
         & $128 \times 64 \times 64 \times 64$ \\
         & $128 \times 128 \times 64 \times 64$ \\
         & $128 \times 128 \times 128 \times 64$ \\
         & $128 \times 128 \times 128 \times 128$ \\
         \bottomrule         
        \end{tabular}   
    }    
\end{table}
\end{comment}

\begin{algorithm}[t]
\caption{Initialization of reordering functions $\order$}\label{algo:initorder}
\SetKwInput{KwInput}{Input}
\SetKwInput{KwOutput}{Output}
\KwInput{a tensor $\tensor{X} \in \mathbb{R}^{\shape}$}
\KwOutput{reordering functions $\order = (\pi_1, \cdots, \pi_d)$}
 \For{$k \leftarrow 1$ \textnormal{to} $d$}{
    \tcp{\small Construct a complete graph}  
    \For{$j \leftarrow 0$ \textnormal{to} $N_k-1$, $h \leftarrow j+1$ \textnormal{to} $N_k-1$\label{algo:initorder:cons:for}}{
        $w(j,h), w(h,j) \leftarrow \fnorm{\slice{i}{j} - \slice{i}{h}}$  \label{algo:initorder:cons:weight}
    }
    \tcp{\small Initialize a tree $T$}  
    $T.root \leftarrow \{\text{a randomly sampled integer from } [N_k]\}$ \label{algo:initorder:tsp:start}\\
    $U \leftarrow [N_k] \setminus T$.nodeset \\    
    \tcp{\small Run Prim's algorithm} 
    \While{$|U| > 0$}   
    {
        $j, h \leftarrow \textnormal{argmin}_{j \in T, h \in U} w(j,h)$  \\
        $T$.$j$.child $\leftarrow$ $T$.$j$.child $\cup$ $\{h\}$ \\
        $U \leftarrow U \setminus \{h\}$
    }
    $P \leftarrow$ DFS$(T)$  \Comment*[f]{\small Depth first search at $T$} \\    
    $P[N_k] \leftarrow P[0]$  \label{algo:initorder:tsp:end}\\
    \tcp{\small Remove the edge with the largest weight}     
    $j \leftarrow \textnormal{argmax}_{j \in [N_k]} w(P[j],P[j+1])$ \label{algo:initorder:remove}\\    
    $\pi_k \leftarrow \texttt{concat}(P[j+1\text{:}N_k], P[0\text{:}j+1])$ \label{algo:initorder:concat}
    %$\pi_k \leftarrow$\\    
 }
 \Return $\order = (\pi_1, \cdots, \pi_d)$
\end{algorithm}

%[TODO: Mention the detailed limitation of TTD connecting C1]}
\label{sec:prelim:TSP}
We introduce the background of the traveling salesman problem (TSP)~\cite{hoffman2013traveling} which is related to formulating the initialization of orders of an input tensor in our model (see details in Section~\ref{sec:method:train:initorder}).
Given a complete loopless undirected graph $G=(V,E)$ with a weight function $w : E \rightarrow \mathbb{R}^{+}$ that maps each edge to a non-negative real value, the TSP problem aims to find a Hamiltonian cycle $H$ that visits each node exactly once such that $w(H)=\sum_{e\in H}w(e)$ is minimized where $V$ and $E$ are the sets of nodes and edges, respectively.

%If the weight function $w$ satisfies the following triangle inequality, the problem is called Metric TSP~\cite{kao2008encyclopedia}:
If the weight function $w$ satisfies the triangle inequality ($w(u,v) \leq w(u,x) + w(x,v), \forall u,v,x \in V$), the problem is called Metric TSP~\cite{kao2008encyclopedia}.
%\begin{equation*}
%    w(u,v) \leq w(u,x) + w(x,v), \forall u,v,x \in V
%\end{equation*}

As Metric TSP belongs to NP-complete, we need approximation algorithms to solve within a certain factor of the optimal answer in polynomial time.
In this work, we consider a 2-approximation algorithm for Metric TSP as follows.
It first computes a minimum spanning tree (MST) $T$ of $G$ and obtains an Eulerian multigraph $T'$ by duplicating each edge of $T$.
After then, it computes an Eulerian tour of $T'$, which is the 2-approximation solution.
The running time of this algorithm is dominated by the computing process of MST which can be earned by Prim's algorithm~\cite{prim1957shortest} whose time complexity is $O(|V|^2)$ when the given graph is complete.

Algorithm~\ref{algo:initorder} describes the detailed process of 
initializing the reordering functions $\order$ using the Metric TSP problem formulation and the 2-approximation solution, which is outlined in Section~\ref{sec:method:reordering}.
